# Supplementary material for: Difference Target Propagation
Source: arXiv:1412.7525 source file (2015-11-25)
Supplement: Supplementary file 1 [file appendix.tex]

\newpage
%\begin{center}
%  {\LARGE APPENDIX}
%\end{center}

% redefine the command that creates the equation no.
\setcounter{equation}{0}  % reset counter 
\section*{\huge Appendix}  % use *-form to suppress numbering

\section{Proof of Proposition 1} \label{app:app1}  

\textbf{Proposition 1.}
\textit{Assume that $g_i$ is a perfect inverse of $f_i$, where $g_i = f_i^{-1}, i=1,...,M-1$ and
$f_i$ satisfies: 1. $f_i$ is a linear mapping or, 2. $\mathbf{h}_i=f_i(\mathbf{h}_{i-1}) = W_is_i(\mathbf{h}_{i-1})$, 
which is another way to obtain a non-linear deep network structure (here $s_i$ can be any differentiable monotonically increasing element-wise function).
Consider one update for both target propagation
and back-propagation,
%the training sample is $(\mathbf{x},\mathbf{y})$,
%and the loss function is $L_{(\mathbf{x}, %\mathbf{y};\mathbf{\theta_W})}$. 
with the target propagation update (with perfect inverse) in $i$th layer being $\delta W_{i}^{tp}$, 
and  the back-propagation update being $\delta W_{i}^{bp}$. 
If the $\hat{eta}$ for assigning the target in 
the highest hidden layer is sufficiently small, then the $cos$ value of angle $\alpha_{i}$ between $\delta W_{i}^{tp}$ and $\delta W_{i}^{bp}$ is bounded by
\begin{equation}
\frac{1+\Delta_1(\hat{\eta})}{\frac{\lambda_{max}}{\lambda_{min}}+\Delta_2(\hat{eta})}
\leq cos(\alpha_{i}) \leq 1
\end{equation}
Here $\lambda_{max}$ and $\lambda_{min}$ are the largest and smallest singular values
of $(J_{f_{M}}\dots J_{f_{i+1}})^T$, where
$J_{f_k}$ is the Jacobian matrix of $f_k$.
$\Delta_1(\hat{eta})$ and $\Delta_2(\hat{\eta})$ are terms propotional to $\hat{\eta}$
when $\hat{\eta}$ is sufficiently small. }

\textit{\textbf{Proof.}} During one update, the training sample is $(\mathbf{x}, \mathbf{y})$,
with assumed $f_i$ we have:
\begin{equation}
\mathbf{h}_i=f_i(\mathbf{h}_{i-1})=W_is_i(\mathbf{h}_{i-1}), i=1,\dots,M
\end{equation}
Here $s_i$ is identity element-wise function if $f_i$ is linear mapping.
According to the loss function in section 2.1, the back-propagation update $\delta W_{i}^{bp}$ is then
\begin{eqnarray}
\nonumber \delta W_{i}^{bp} &=& -\eta_{bp}\frac{\partial L(\mathbf{x}, \mathbf{y};\mathbf{\theta}_W^{0,M})}{\partial W_i} \\
\nonumber &=& -\eta_{bp}(\frac{\partial\mathbf{h}_{i+1}}{\partial\mathbf{h}_i})^T \dots (\frac{\partial \mathbf{h}_{M}}{\partial \mathbf{h}_{M-1}})^T \frac{\partial L}{\partial \mathbf{h}_{M}}(s_i(\mathbf{h}_{i-1}))^T \\
&=& -\eta_{bp}J_{f_{i+1}}^T \dots J_{f_{M}}^T \frac{\partial L}{\partial \mathbf{h}_{M}}(s_i(\mathbf{h}_{i-1}))^T
\end{eqnarray}
where
\begin{equation}
J_{f_k}=\frac{\partial \mathbf{h}_{k}}{\partial \mathbf{h}_{k-1}} = W_i \cdot S_i'(\mathbf{h}_{k-1}), k=i+1,\dots,M
\end{equation}
$S_i'(\mathbf{h}_{k-1})$ is a diagonal matrix with each diagonal element being corresponding element-wise derivatives and $J_{f_k}$ is the Jocobian matirx of $f_k(\mathbf{h}_{k-1})$ with respect to $\mathbf{h}_{i-1}$.

Target propagation update is more complicated.
For layer $M$, target $\hat{\mathbf{h}}_{M}$ of $\mathbf{h}_{M}$ is assigned by
\begin{equation}
\hat{\mathbf{h}}_{M} = \mathbf{h}_{M} - \hat{\eta}\frac{\partial L}{\partial \mathbf{h}_{M}}
\end{equation}
If all $\mathbf{h}_k$s are allocated in smooth areas and $\hat{\eta}$ is sufficiently small, then the target $\hat{\mathbf{h}}_i$ in
layer $i$ is achieved by perfect inverse $g_k=f_k^{-1}, k=i+1,\dots,M$ with Taylor expansion that
\begin{eqnarray}
\nonumber \hat{\mathbf{h}}_i &=& g_{i+1}(\dots g_{M}(\hat{\mathbf{h}}_{M})\dots) \\
&=& g_{i+1}(\dots g_{M}(\mathbf{h}_{M})\dots) - \hat{\eta} J_{g_{i+1}}\dots J_{g_{M}}\frac{\partial L}{\partial \mathbf{h}_{M}}+\mathbf{o}(\hat{\eta}^2)
%&\simeq&\mathbf{h}_i-\eta_0 J_{f_{i+1}}^{-1}\dots J_{f_{M-1}}^{-1}\frac{\partial loss(\mathbf{h}_M, y)}{\partial \mathbf{h}_{M-1}}
\end{eqnarray}

Here $\mathbf{o}(\hat{\eta}^2)$ is a vector including the higher order term and it has the same size as $\hat{\mathbf{h}}_{M}$.  Now for target propagation update $\delta W_{i}^{tp}$ we have
\begin{eqnarray}
\nonumber \delta W_{i}^{tp} &=& -\eta_{tp}\frac{\partial||\mathbf{h}_i(\mathbf{h}_{i-1};W_i)-\hat{\mathbf{h}}_i||^2_2}{\partial W_i}\\
\nonumber &=& - \eta_{tp}(\mathbf{h}_i-(\mathbf{h}_i-\hat{\eta} J_{f_{i+1}}^{-1}\dots J_{f_{M}}^{-1}\frac{\partial L}{\partial \mathbf{h}_{M}}+\mathbf{o}(\hat{\eta}^2)))(s_i(\mathbf{h}_{i-1}))^T\\ 
&=& - \eta_{tp}\hat{\eta}J_{f_{i+1}}^{-1}\dots J_{f_{M}}^{-1}\frac{\partial L}{\partial \mathbf{h}_{M}}(s_i(\mathbf{h}_{i-1}))^T +\eta_{tp}\mathbf{o}(\hat{\eta}^2) (s_i(\mathbf{h}_{i-1}))^T
\end{eqnarray}
here we write $\frac{\partial L}{\partial \mathbf{h}_{M}}$ as $\textit{\textbf{l}}$
, $s_i(\mathbf{h}_{i-1})$ as \textit{\textbf{v}} and $J_{f_{M}}\dots J_{f_{i+1}}$ as $J$ for short. Since $\delta W_{i}^{bp}$ and $\delta W_{i}^{tp}$ are in matrix form, the inner production of their vector forms $vec(\delta W_{i}^{bp})$ and $vec(\delta W_{i}^{tp})$ is
\begin{eqnarray}
\nonumber &&\langle vec(\delta W_{i}^{bp}), vec(\delta W_{i}^{tp}) \rangle \\ %&=& tr((\delta W_{i}^{bp})^T\delta W_{i}^{tp})\\
\nonumber &=& tr((-\eta_{bp}J^T \textit{\textbf{l}}\textit{\textbf{v}}^T)^T(-\eta_{tp}\hat{\eta}J^{-1} \textit{\textbf{l}}\textit{\textbf{v}}^T + \eta_{tp}\mathbf{o}(\hat{\eta}^2) \textit{\textbf{v}}^T))\\
\nonumber &=& \eta_{bp}\eta_{tp}\hat{\eta}tr(\textit{\textbf{v}}\textit{\textbf{l}}^TJJ^{-1} \textit{\textbf{l}}\textit{\textbf{v}}^T)
- \eta_{bp}\eta_{tp}tr(\textit{\textbf{v}}\textit{\textbf{l}}^TJ\mathbf{o}(\hat{\eta}^2)\textit{\textbf{v}}^T)\\
\nonumber &=&\eta_{bp}\eta_{tp}\hat{\eta}tr(\textit{\textbf{v}}\textit{\textbf{l}}^T\textit{\textbf{l}}\textit{\textbf{v}}^T)
- \eta_{bp}\eta_{tp}tr(\textit{\textbf{l}}^TJ\mathbf{o}(\hat{\eta}^2))||\textit{\textbf{v}}||^2_2\\
&=&\eta_{bp}\eta_{tp}\hat{\eta}||\textit{\textbf{v}}||^2_2\cdot||\textit{\textbf{l}}||^2_2
- \eta_{bp}\eta_{tp}\langle J^T\textit{\textbf{l}}, \mathbf{o}(\hat{\eta}^2)\rangle||\textit{\textbf{v}}||^2_2
\end{eqnarray}
Also for $||vec(\delta W_{i}^{bp})||_2$ and $||vec(\delta W_{i}^{tp})||_2$ we have
\begin{eqnarray}
 ||vec(\delta W_{i}^{bp})||_2 %&=& tr((\delta W_{i}^{bp})^T\delta W_{i}^{tp})\\
\nonumber &=& \sqrt{tr((-\eta_{bp}J^T \textit{\textbf{l}}\textit{\textbf{v}}^T)^T(-\eta_{bp}J^T \textit{\textbf{l}}\textit{\textbf{v}}^T))}\\
\nonumber &=& \eta_{bp} \sqrt{tr(\textit{\textbf{v}}(J^T \textit{\textbf{l}})^T (J^T \textit{\textbf{l}})\textit{\textbf{v}}^T)}\\
\nonumber &=&\eta_{bp}||\textit{\textbf{v}}||_2\cdot||J^T \textit{\textbf{l}}||_2\\
&\leq& \eta_{bp}||\textit{\textbf{v}}||_2\cdot||J^T||_2\cdot||\textit{\textbf{l}}||_2
\end{eqnarray}
and similarly,
\begin{eqnarray}
 ||vec(\delta W_{i}^{tp})||_2 %&=& tr((\delta W_{i}^{bp})^T\delta W_{i}^{tp})\\
&\leq& \eta_{tp}\hat{\eta}||\textit{\textbf{v}}||_2\cdot||J^{-1}||_2\cdot||\textit{\textbf{l}}||_2
+\eta_{tp}||\mathbf{o}(\hat{\eta}^2)||_2\cdot||\textit{\textbf{v}}||_2
\end{eqnarray}
here $||J^T||_2$ and $||J^{-1}||_2$ are matrix Euclidian norms,
i.e. the largest singular value of $(J_{f_{M}}\dots J_{f_{i+1}})^T$, $\lambda_{max}$,
				and the largest singular value of $(J_{f_{M}}\dots J_{f_{i+1}})^{-1}$, $\frac{1}{\lambda_{min}}$
				($\lambda_{min}$ is the smallest singular value of $(J_{f_{M}}\dots J_{f_{i+1}})^T$,
				 because $f_k$ is invertable, so all the smallest singular values of Jacobians are larger than $0$).
Finally, if $\hat{\eta}$ is sufficiently small, the angle $\alpha_i$ between $vec(\delta W_{i}^{bp})$ and $vec(\delta W_{i}^{tp})$ satisfies:
\begin{eqnarray}
\nonumber cos(\alpha_i) &=& \frac{\langle vec(\delta W_{i}^{bp}), vec(\delta W_{i}^{tp}) \rangle}{||vec(\delta W_{i}^{bp})||_2\cdot||vec(\delta W_{i}^{tp})||_2}\\
\nonumber &\geq& \frac{\eta_{bp}\eta_{tp}\hat{\eta}||\textit{\textbf{v}}||^2_2||\textit{\textbf{l}}||^2_2
- \eta_{bp}\eta_{tp}\langle J^T\textit{\textbf{l}}, \mathbf{o}(\hat{\eta}^2)\rangle||\textit{\textbf{v}}||^2_2}
{(\eta_{bp}||\textit{\textbf{v}}||_2\lambda_{max}||\textit{\textbf{l}}||_2)
(\eta_{tp}\hat{\eta}||\textit{\textbf{v}}||_2(\frac{1}{\lambda_{min}})||\textit{\textbf{l}}||_2
+\eta_{tp}||\mathbf{o}(\hat{\eta}^2)||_2||\textit{\textbf{v}}||_2)}\\
\nonumber &=& \frac{1+\frac{- \langle J^T\textit{\textbf{l}}, \mathbf{o}(\hat{\eta}^2)\rangle}{\hat{\eta}||\textit{\textbf{l}}||^2_2}}
{\frac{\lambda_{max}}{\lambda_{min}}+\frac{\lambda_{max}||\mathbf{o}(\hat{\eta}^2)||_2}{\hat{\eta}||\textit{\textbf{l}}||_2}}\\
&=& \frac{1+\Delta_1(\hat{\eta})}
{\frac{\lambda_{max}}{\lambda_{min}}+\Delta_2(\hat{\eta})}
\end{eqnarray}
and $cos(\alpha_i)\leq 1$ is trivial.\hfill$\square$

\newpage
\section{Proof of Proposition 2}

\textbf{Proposition 2.}
\textit{During the $t+1$ th update in difference target propagation, we use $L_i^{inv}(\hat{\mathbf{h}}_i^{(t)} + \mathbf{\epsilon};V_i,W_i^{(t)})$ to update $V_i^{(t+1)}$ and we
define $\bar{L}_i^{inv}(V_i,W_i^{(t)})$ as the expected local auto-encoder-like
loss function over all possible $\hat{\mathbf{h}}_i^{(t)}+\mathbf{\epsilon}$ with $W_i^{(t)}$ fixed,
\begin{equation}
\bar{L}_i^{inv}(V_i,W_i^{(t)}) = \mathop{\mathbb{E}}_{\hat{\mathbf{h}}_{i}^{(t)}, \mathbf{\epsilon}}\{L_i^{inv}(\hat{\mathbf{h}}_{i}^{(t)}+\mathbf{\epsilon};V_i,W_i^{(t)})\}
\end{equation}
If 1.$\bar{L}_i^{inv}(V_i,W_i^{(t)})$ has only one
minimum with optimal $V_{i}^{*}(W_i^{(t)})$; 2. proper learning rates for
$V_i$ and $W_i$ are given; 3. All the Jacobian and Hessian like matrices are
bounded during learning; 4. $\nabla_{V_i}\bar{L}_i^{inv}(V_i,W_i^{(t)})$
always points towards optimal $V_{i}^{*}(W_i^{(t)})$;
5. $\mathop{\mathbb{E}}\{V_i^{*}(W_i^{(t+1)})-V_i^{*}(W_i^{(t)}) \mid W_i^{(t)} \}=0$.
Then $V_i^{(t)}-V_{i}^{*}(W_i^{(t)})$ will almost surely converge
to $0$ at $t$ th update when $t$ goes to infinity. Condition 1, 2, 4
follow the settings of stochastic gradient descent convergence similar to ~\citep{bottou-98x}.
}

\textit{\textbf{Proof.}}
%The proof follows the work in \citep{bottou}. 
Let us first give detail explanation for condition 2, 3, 4.
For condition 2, proper learning rates $\eta_v$ and $\eta_w$ satisfy
\begin{equation}
\label{lr_bound0}
\sum_{t=1}^{\infty}{\eta_v^{(t)}(\eta_w^{(t)}) = +\infty }, \sum_{t=1}^{\infty}{(\eta_v^{(t)})^2((\eta_w^{(t)})^2) < +\infty }
\end{equation}
Note that the the beginning learning rate $\eta_v^{(1)}(\eta_w^{(1)})$ can be assigned as $\frac{1}{n_0}$ to be sufficiently small to satisfy locally smooth condition if needed.
Condition 3 basically says that the norm of first order terms like
$\nabla_{V_i} L_i^{inv}(\hat{\mathbf{h}}_{i}+\mathbf{\epsilon};V_i,W_i)$
and $\nabla_{W_i}L_i(W_i)$ which are special cases of Jacobians, and eigenvalues of second order terms like
$\frac{\partial^2 L_i^{inv}(\hat{\mathbf{h}}_{i}+\mathbf{\epsilon};V_i,W_i)}{\partial V_i^2}$,
$\frac{\partial^2 L_i^{inv}(\hat{\mathbf{h}}_{i}+\mathbf{\epsilon};V_i,W_i)}{\partial V_i\partial W_i}$ are bounded.
%This condition is easily satisfied if the activition function is like $tanh(\cdot)$ or $sigmoid(\cdot)$.
Codition 4 is equavilent to the following
\begin{equation}
\forall \varepsilon>0, \mathop{inf}_{||V_i-V_{i}^{*}(W_i^{(t)})||_2>\varepsilon}(V_i-V_{i}^{*}(W_i^{(t)}))^T\nabla_{V_i}\bar{L}_i^{inv}(V_i,W_i^{(t)})>0
\end{equation}
above condition basically says that oppoite of the gradient $-\nabla_{V_i}\bar{L}_i^{inv}(V_i,W_i^{(t)})$ always at least partly points towards its minimum with optimal $V_{i}^{*}(W_i^{(t)})$.

Note that in the following proof, all $V_i$s and $W_i$s are in \textit{vector form}.
$V_i^{(t)}$ and  $W_i^{(t)}$ follow their update rules like
\begin{equation}
V_i^{(t+1)}=V_i^{(t)}-\eta_v^{(t)}\nabla_{V_i} L_i^{inv}(\hat{\mathbf{h}}_{i}^{(t)}+\mathbf{\epsilon};V_i,W_i^{(t)})
\end{equation}
\begin{equation}
W_i^{(t+1)}=W_i^{(t)}-\eta_w^{(t)}\delta W_i^{(t)}
\end{equation}
$\delta W_i^{(t)}$ respects to $\nabla_{W_i}L_i(W_i)$ in difference target propagation.
We define $\gamma_t$ that
\begin{equation}
\gamma_t = ||V_i^{(t)}-V_{i}^{*}(W_i^{(t)})||_2^2
\end{equation}
The $\gamma_t$ measures how far the current $V_i^{(t)}$ is from the optimum.
During the learning process, the randomness is only introduced by every update's sample $(\mathbf{x},\mathbf{y})$ and
the $\epsilon$ used in updating $V_i$. 
We care about whether $\gamma_t$ converges and we check the following conditional expcation
\begin{eqnarray}
\nonumber &&\mathbb{E}\{\gamma_{t+1}-\gamma_t \mid V_i^{(t)}, W_i^{(t)}\}\\ 
\nonumber &=&\mathbb{E}\{||V_i^{(t)}-\eta_v^{(t)}\nabla_{V_i} L_i^{inv}(\hat{\mathbf{h}}_{i}^{(t)}+\mathbf{\epsilon};V_i,W_i^{(t)})-V_{i}^{*}(W_i^{(t+1)})||_2^2\\
\nonumber&&-||V_i^{(t)}-V_{i}^{*}(W_i^{(t)})||_2^2 \mid  V_i^{(t)}, W_i^{(t)}\}\\
 \nonumber&=& -2\eta_v^{(t)}(V_{i}^{(t)}- V_{i}^{*}(W_i^{(t)}))^T\mathop{\mathbb{E}}_{\hat{\mathbf{h}}^{(t)}_i,\epsilon}\{\nabla_{V_i} L_i^{inv}(\hat{\mathbf{h}}_{i}^{(t)}+\mathbf{\epsilon};V_i,W_i^{(t)})\}\\
 \nonumber&&+(\eta_v^{(t)})^2\mathop{\mathbb{E}}_{\hat{\mathbf{h}}^{(t)}_i,\epsilon}\{||\nabla_{V_i} L_i^{inv}(\hat{\mathbf{h}}_{i}^{(t)}+\mathbf{\epsilon};V_i,W_i^{(t)})||^2_2\}\\
\label{term1}
&& + 2(V_i^{(t)}-V_{i}^{*}(W_i^{(t)}))^T\mathbb{E}\{V_{i}^{*}(W_i^{(t)})- V_{i}^{*}(W_i^{(t+1)})\mid W_i^{(t)}\}\\
	\nonumber&&- 2\eta_v^{(t)}\mathop{\mathbb{E}}_{\hat{\mathbf{h}}^{(t)}_i, \epsilon}\{(\nabla_{V_i} L_i^{inv}(\hat{\mathbf{h}}_{i}^{(t)}+\mathbf{\epsilon};V_i,W_i^{(t)}))^T(V_{i}^{*}(W_i^{(t)})- V_{i}^{*}(W_i^{(t+1)})\mid W_i^{(t)}\}\\
 \nonumber&& + \mathbb{E}\{||V_{i}^{*}(W_i^{(t)})- V_{i}^{*}(W_i^{(t+1)})||^2_2 \mid W_i^{(t)}\}\\
&=& -2\eta_v^{(t)}(V_{i}^{(t)}- V_{i}^{*}(W_i^{(t)}))^T\nabla_{V_i} \bar{L}_i^{inv}(V_i^{(t)},W_i^{(t)})\\
\label{term2}
 &&+(\eta_v^{(t)})^2\mathop{\mathbb{E}}_{\hat{\mathbf{h}}^{(t)}_i,\epsilon}\{||\nabla_{V_i} L_i^{inv}(\hat{\mathbf{h}}_{i}^{(t)}+\mathbf{\epsilon};V_i,W_i^{(t)})||^2_2\}\\
 \label{term3}
	&&- 2\eta_v^{(t)}\mathop{\mathbb{E}}_{\hat{\mathbf{h}}^{(t)}_i, \epsilon}\{(\nabla_{V_i} L_i^{inv}(\hat{\mathbf{h}}_{i}^{(t)}+\mathbf{\epsilon};V_i,W_i^{(t)}))^T(V_{i}^{*}(W_i^{(t)})- V_{i}^{*}(W_i^{(t+1)})\mid W_i^{(t)}\}\\
\label{term4}
&& + \mathbb{E}\{||V_{i}^{*}(W_i^{(t)})- V_{i}^{*}(W_i^{(t+1)})||^2_2 \mid W_i^{(t)}\}
\end{eqnarray}
We can see that term (\ref{term1}) is cancelled by condition 5. In term (\ref{term2}), because
the norm of $\nabla_{V_i} L_i^{inv}(\hat{\mathbf{h}}_{i}+\mathbf{\epsilon};V_i,W_i)$
is bounded by some non-negative constant $\alpha_{v}$, we have
\begin{equation}
\label{bound1}
\mathop{\mathbb{E}}_{\hat{\mathbf{h}}_i,\epsilon}\{||\nabla_{V_i} L_i^{inv}(\hat{\mathbf{h}}_{i}+\mathbf{\epsilon};V_i,W_i^{(t)})||^2_2\} \leq \alpha_{v}^2
\end{equation}
Let us check term (\ref{term3}) and term (\ref{term4}) where both
of them have the term
\begin{equation}
\Delta^* = V_{i}^{*}(W_i^{(t)})- V_{i}^{*}(W_i^{(t+1)})
\end{equation}
Because $V_{i}^{*}(W_i^{(t)})$ is the optimum minimizing $\bar{L}_i^{inv}(V_{i},W_i^{(t)})$, we have
\begin{eqnarray}
\label{optimal_diff}
\nonumber \mathbf{0} &=& \nabla_{V_i} \bar{L}_i^{inv}(V_{i}^{*}(W_i^{(t)}),W_i^{(t)})\\
\nonumber &=& \nabla_{V_i} \bar{L}_i^{inv}(V_{i}^{*}(W_i^{(t+1)}),W_i^{(t+1)})\\
&=& \nabla_{V_i} \bar{L}_i^{inv}(V_{i}^{*}(W_i^{(t)})-\Delta^*,W_i^{(t)}-\eta^{(t)}_w\delta W_i^{(t)}) 
\end{eqnarray}
If the learning rate for $V_i$ and $W_i$ is small enough with local smoothness satisfied, we can transform Eq.\ref{optimal_diff} like
\begin{equation}
\label{deltastar}
\mathbf{0} =-\frac{\partial^2 \bar{L}_i^{inv}(V_i,W_i)}{\partial V_i^2}\Delta^*
-\eta^{(t)}_w\frac{\partial^2 \bar{L}_i^{inv}(V_i,W_i)}{\partial V_i\partial W_i}\delta W^{(t)}_i
+\mathbf{o}(||\Delta^*||_2^2) + \mathbf{o}(||\eta^{(t)}_w\delta W^{(t)}_i||^2_2)
\end{equation}
Here $||\mathbf{o}(||\Delta^*||_2^2)||_2\leq\varepsilon_{\Delta}||\Delta^*||_2$
and $||\mathbf{o}(||\eta^{(t)}_w\delta W^{(t)}_i||^2_2)||_2\leq \varepsilon_{w}||\eta^{(t)}_w\delta W^{(t)}_i||_2 $ for local smoothness.
With the fact that all the second order terms are bounded, based on Eq.\ref{deltastar} we have
\begin{equation}
||\Delta^*||_2 \leq \alpha_{\Delta}\eta^{(t)}_w||\delta W^{(t)}_i||_2
\end{equation}
Here $\alpha_{\Delta}$ is some non-negative constant. Further more,
because the first order term of $W_i$ like $\nabla_{W_i}L_i(W_i)$ is also bounded, we have 
\begin{equation}
||\delta W^{(t)}_i||_2\leq \alpha_{w}
\end{equation}
Here $\alpha_{w}$ is some non-negative constant.
Now for term (\ref{term3}) we have
\begin{eqnarray}
|\mathop{\mathbb{E}}_{\hat{\mathbf{h}}^{(t)}_i, \epsilon}\{(\nabla_{V_i} L_i^{inv}(\hat{\mathbf{h}}_{i}^{(t)}+
\mathbf{\epsilon};V_i,W_i^{(t)}))^T(V_{i}^{*}(W_i^{(t)})- V_{i}^{*}(W_i^{(t+1)})\mid W_i^{(t)}\}|\leq
\alpha_{\Delta}\alpha_{v}\alpha_{w}\eta^{(t)}_w
\end{eqnarray}
and the absolute value of the entire term (\ref{term3}) is then bounded by
\begin{equation}
2\alpha_{\Delta}\alpha_{v}\alpha_{w}\eta^{(t)}_w\eta^{(t)}_v
\end{equation}
Based on \textit{Cauthy-Schwarz inequality}, $\eta^{(t)}_w\eta^{(t)}_v$ satisfies
\begin{equation}
(\sum_{t=1}^{N}\eta^{(t)}_w\eta^{(t)}_v)^2\leq(\sum_{t=1}^{N}(\eta^{(t)}_w)^2)(\sum_{t=1}^{N}(\eta^{(t)}_v)^2)
\end{equation}
From the learning rates condition, we know that
\begin{equation}
\lim_{N \to \infty}\sum_{t=1}^{N}{(\eta_w^{(t)})^2((\eta_v^{(t)})^2) < +\infty }
\end{equation}
Because $\eta^{(t)}_w$ and $\eta^{(t)}_v$ are positive, then we can easily have
\begin{equation}
\label{lr_bound}
\lim_{N \to \infty}\sum_{t=1}^{N}{\eta^{(t)}_w\eta^{(t)}_v < +\infty }
\end{equation}
For term (\ref{term4}) we have
\begin{equation}
 \mathbb{E}\{||V_{i}^{*}(W_i^{(t)})- V_{i}^{*}(W_i^{(t+1)})||^2_2 \mid W_i^{(t)}\}\leq \alpha_{\Delta}^2\alpha_{w}^2(\eta^{(t)}_w)^2
\end{equation}
Finally, $\mathbb{E}\{\gamma_{t+1}-\gamma_t \mid V_i^{(t)}, W_i^{(t)}\}$ satisfies
\begin{eqnarray}
\label{expaction_bound}
\nonumber &&\mathbb{E}\{\gamma_{t+1}-\gamma_t \mid V_i^{(t)}, W_i^{(t)}\} \\
\nonumber &\leq&-2\eta_v^{(t)}(V_{i}^{(t)}- V_{i}^{*}(W_i^{(t)}))^T\nabla_{V_i} \bar{L}_i^{inv}(V_i^{(t)},W_i^{(t)})\\
\nonumber &&+(\eta^{(t)}_v)^2(\alpha_v)^2 +2\alpha_{\Delta}\alpha_{v}\alpha_{w}\eta^{(t)}_w\eta^{(t)}_v+ \alpha_{\Delta}^2\alpha_{w}^2(\eta^{(t)}_w)^2\\ 
&\leq& (\eta^{(t)}_v)^2(\alpha_v)^2 +2\alpha_{\Delta}\alpha_{v}\alpha_{w}\eta^{(t)}_w\eta^{(t)}_v+ \alpha_{\Delta}^2\alpha_{w}^2(\eta^{(t)}_w)^2 
\end{eqnarray}
From Eq.\ref{lr_bound0} and Eq.\ref{lr_bound}, we know that the right side of Eq.\ref{expaction_bound} is the summand of a convergent
infinite sum.
Since process $\{\gamma_t\}$ always larger than $0$,
and Eq.\ref{expaction_bound} gives the upper bound of positive expected variation of $\gamma_t$,
from \textit{Quasi-martingale convergence theorem} in section 4.4 of \citep{bottou-98x},
we have that $\gamma_t$ converges amlost surely.
The almost surely convergence of $\gamma_t$ and Eq.\ref{expaction_bound} imply that
\begin{equation}
\sum_{t=1}^{\infty}{\eta_v^{(t)}(V_{i}^{(t)}- V_{i}^{*}(W_i^{(t)}))^T\nabla_{V_i} \bar{L}_i^{inv}(V_i^{(t)},W_i^{(t)})} \leq +\infty, \quad a.s.
\end{equation}
Here \textit{a.s.} means \textit{almost surely}. With the learning rate $\eta_v^{(t)}$ satisfies
\begin{equation}
\sum_{t=1}^{\infty}{\eta_v^{(t)}} = +\infty
\end{equation}
and $(V_{i}^{(t)}- V_{i}^{*}(W_i^{(t)}))^T\nabla_{V_i} \bar{L}_i^{inv}(V_i^{(t)},W_i^{(t)})$ is always positive because of condition 4,
we have 
\begin{equation}
\label{limit}
\lim_{t \to \infty}{(V_{i}^{(t)}- V_{i}^{*}(W_i^{(t)}))^T\nabla_{V_i} \bar{L}_i^{inv}(V_i^{(t)},W_i^{(t)}) = 0}, \quad a.s.
\end{equation}
Assume that $\gamma_t$ converges to some positive constant rather than $0$.
It implies that when $t$ is large enough,
$\gamma_t = ||V_{i}^{(t)}- V_{i}^{*}(W_i^{(t)})||_2^2 > \varepsilon > 0$.
This is incompatible with condition 3 and Eq.\ref{limit}.
Therefore $\gamma_t$ converges to $0$ almost surely and we have
\begin{equation}
\lim_{t \to \infty}{V_{i}^{(t)}- V_{i}^{*}(W_i^{(t)})=0}, \quad a.s.
\end{equation}
\hfill$\square$

%\end{document}
